# Supplementary material for: Colour and logarithmic accuracy in final-state parton showers
Source: arXiv:2011.10054 source file (2020-11-19)

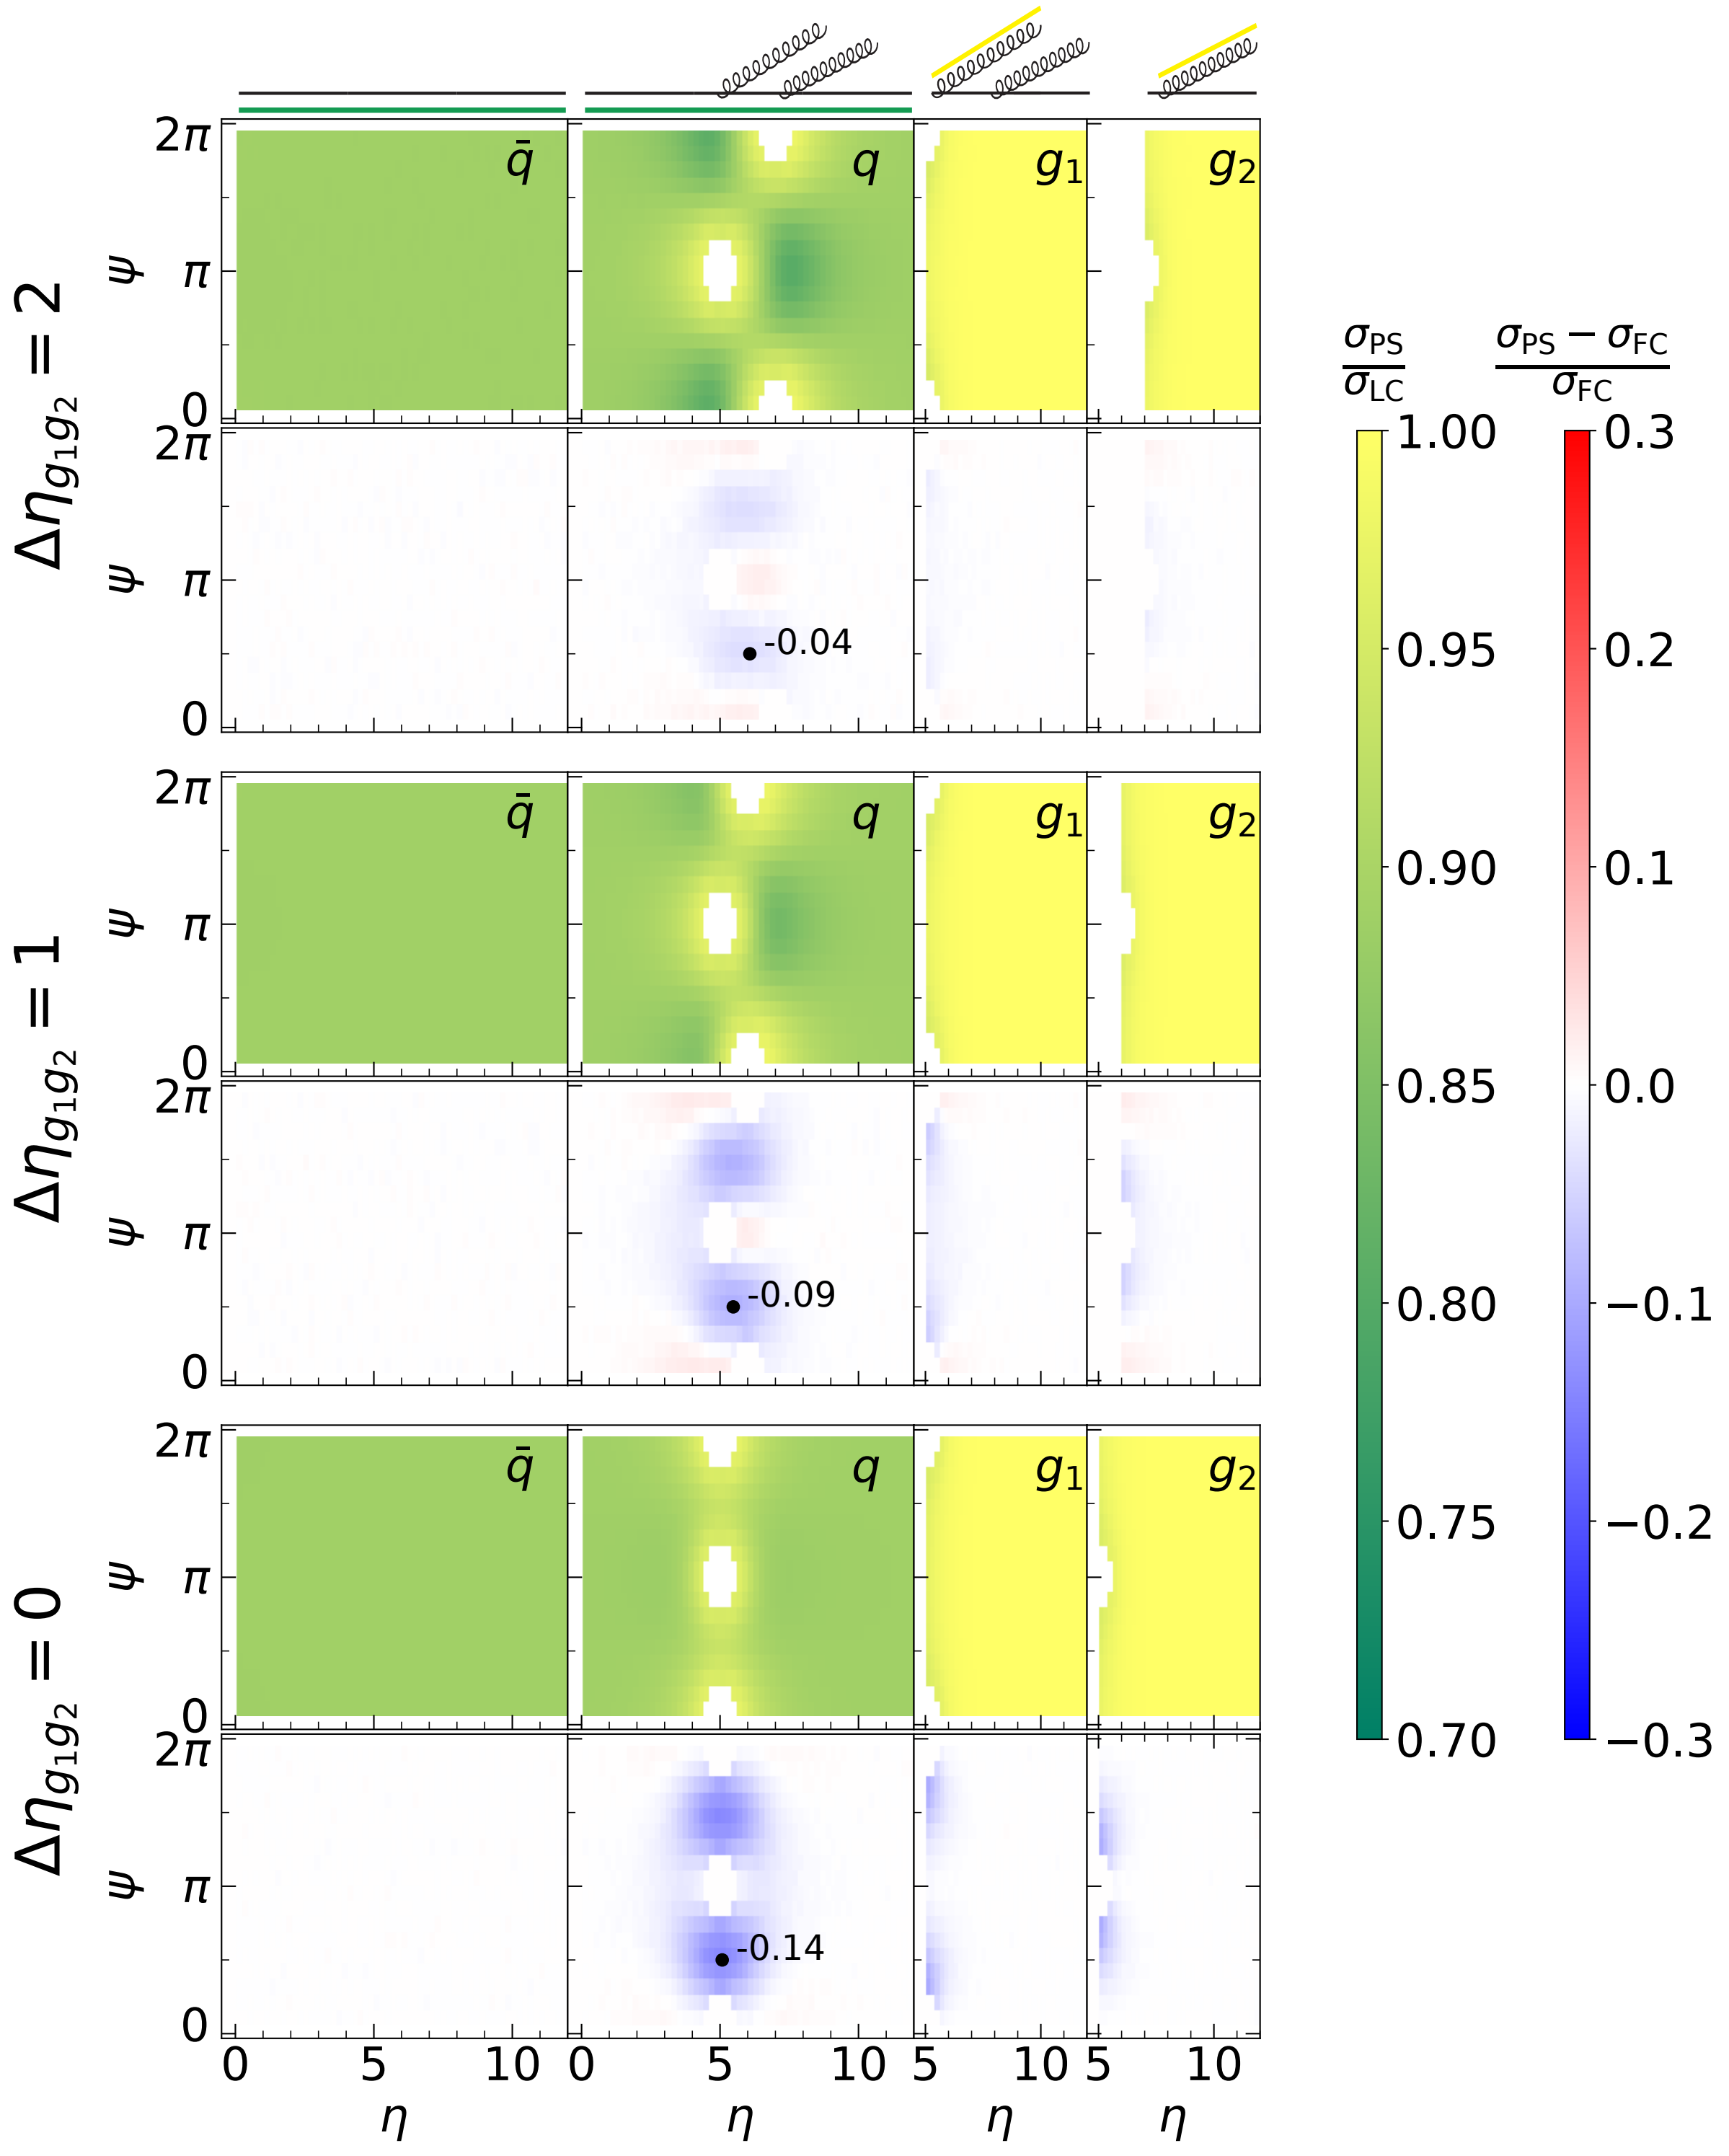

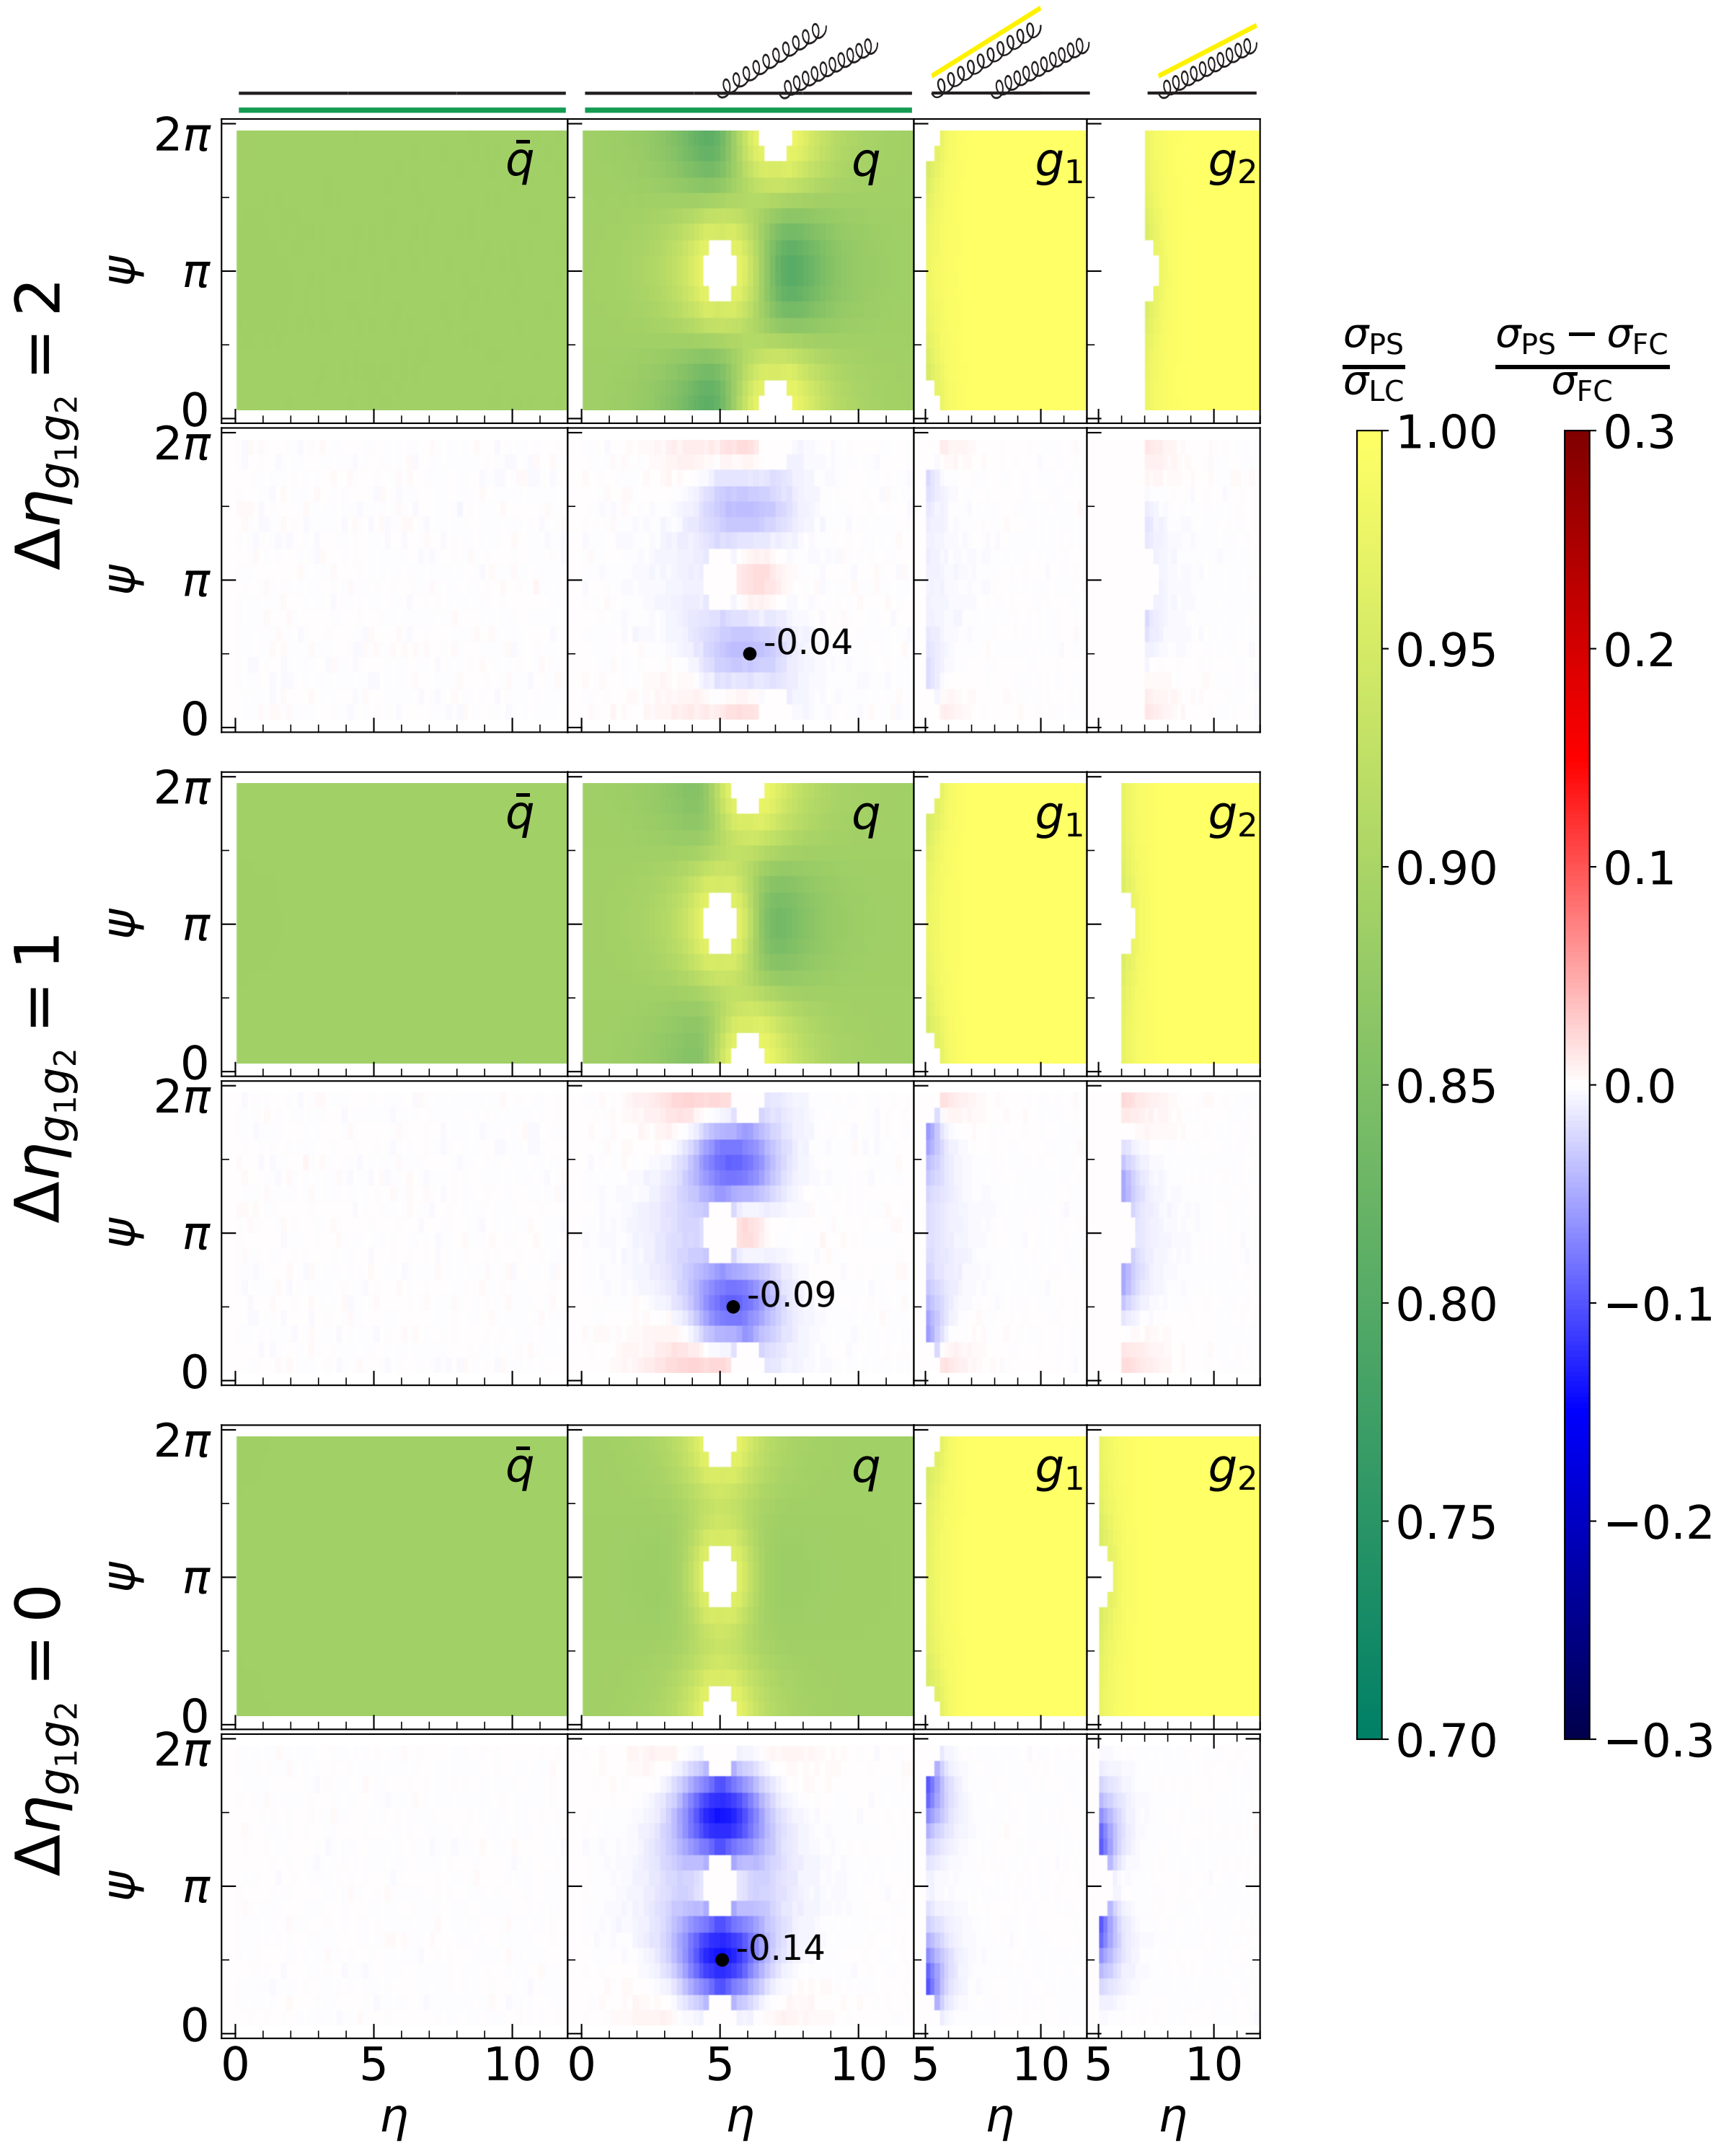

Supplement: Supplementary file 1 [file twod-colour-me-results-appendix-A_wdiagrams.pdf]
